# Supplementary material for: Explaining a machine learning decision to physicians via counterfactuals
Source: arXiv:2306.06325 source file (2023-06-10)
Supplement: Supplementary file 1 [file PPGsynth.tex]

\newpage
\section{Experiments on a synthetic PPG dataset}
\label{sec:ppgsynth}

We show some preliminary results from the CF VAE trained on a synthetic PPG dataset in this section.  

\subsection{Classification task}
We consider the task of classifying regular PPG beats vs premature atrial contraction (PAC). In our experiments, we use a specific type of irregularity in PPG that is `reset'~\cite{tang2020ppgsynth}.

\cite{tang2020ppgsynth} describes a model for a PPG signal which represents heartbeats using two Gaussian functions each. Each time-series is parameterized by the locations of the centers of the Gaussians ($\theta$), the amplitudes ($a$) , the widths ($b$), and the durations of the beats ($d$). 
We represent each PPG signal with these parameters ($a, \theta, b, d$) for each beat.  

For our experiments, we use this model to generate PPG signals of two types: regular and reset.
% This model is used to generate both regular PPG signals and signals with reset.

\subsection{Counterfactuals produced}

We train a neural network with linear layers on this task and achieve an accuracy of 93\%. We then train a CF VAE to generate counterfactual PPG parameters. The goal here would be - given a regular PPG signal, the CF VAE produces a signal with PAC and vice versa. 
Note: the PPG signals are represented using the parameters ($a, \theta, b, d$) as described in~\cite{tang2020ppgsynth}. The CF VAE produces the parameters of a counterfactual PPG signal that we visualize here. 
Some examples of counterfactuals produced by CF VAE are shown in Figures~\ref{fig:ppgeg_1},
~\ref{fig:ppgeg_2},~\ref{fig:ppgeg_3}. 

\begin{figure}[h]
    \centering
    \includegraphics{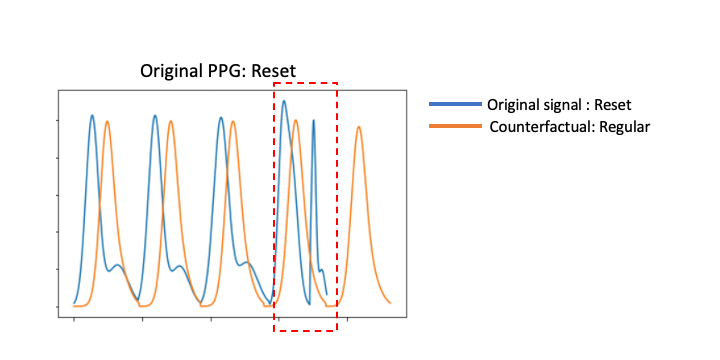}
    \caption{A PPG classification model classifies the original signal shown in blue to have PAC (reset). The region where the irregularity is observed is highlighted. The orange signal is a PPG signal generated by our CF VAE which is a signal that would be classified as a regular PPG.}
    \label{fig:ppgeg_1}
\end{figure}

\begin{figure}[h]
    \centering
    \includegraphics{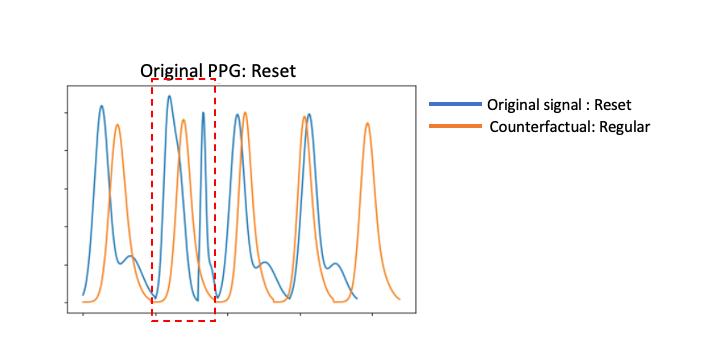}
    \caption{A PPG classification model classifies the original signal shown in blue to have PAC (reset). The region where the irregularity is observed is highlighted. The orange signal is a PPG signal generated by our CF VAE which is a signal that would be classified as a regular PPG.}
    \label{fig:ppgeg_2}
\end{figure}

\begin{figure}[h]
    \centering
    \includegraphics{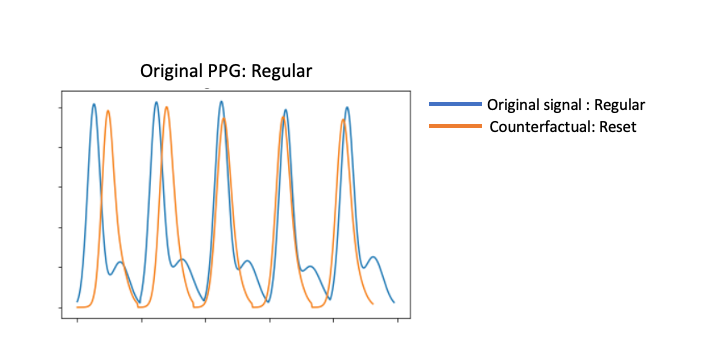}
    \caption{A PPG classification model classifies the original signal shown in blue to be regular. The orange signal is a PPG signal generated by our CF VAE which is a signal that would be classified to have PAC (reset). We can observe here that the orange beats are not as regularly spaced as the one in blue. 
    }
    \label{fig:ppgeg_3}
\end{figure}
