# Supplementary material for: Explaining a machine learning decision to physicians via counterfactuals
Source: arXiv:2306.06325 source file (2023-06-10)
Supplement: Supplementary file 4 [file literature_survey.tex]

\section{Literature Survey}
\label{sec:lit_survey}
%While clinical prediction tasks based on datasets such as MIMIC III have been widely-studied, we believe we are the first to define and tackle the home hospital problem via machine learning methods that leverage the MIMIC III dataset. This is a potentially significant contribution, as home hospital requires the solution to a challenging prediction task, and yet the datasets used by clinical sites in designing home hospital programs and protocols are not generally available to the ML research community, preventing the development of innovative methods which could potentially improve the cost and quality of care. In contrast, prior publications on the home hospital problem~\citep{levine2021hospital,leff2005hospital} in the clinical literature tend to describe point solutions for a particular site or address healthcare-system aspects of the problem. No prior works have defined a computational task on a publicly-available dataset and provided suitable baseline methods. We hope that this work will enable ML health researchers to develop innovative solutions to a pressing modern healthcare system challenge.

%A second contribution of this work is a VAE-based deep architecture for the home hospital problem. Our approach addresses the three main tasks of counterfactual generation, intervention prediction, and patient ranking. We discuss related work for each of these tasks below.

%%We discuss three streams of relevant work: 1) clinical explainable methods in machine learning and predicting in-hospital clinical events.

There is vast existing literature on Explainable AI. Comprehensive surveys include~\citep{adadi2018peeking,abdul2018trends,doshi2017towards}, as well as~\citep{tjoa2020survey} which focuses specifically on clinical settings. 
% \jrnote{Move this to bottom as we want to dive right into the method that matters for us}
%For the home hospital problem, when an algorithm recommends that a patient is a good candidate for home hospital care, we seek to help a physician probe the boundary of the learned model: what about the patient’s vital signs would have to change in order for the model to recommend that the patient remain in the hospital.  
%% removed because seemed redundant with intro
%%Another way to explain an ML model is via a counterfactual. This work was initially motivated by fairness considerations: if a person is denied a loan, what would they have to change in order to qualify?   There is an emphasis on generating diverse counterfactuals capturing the many minimal ways one could improve their credit record, income, etc in order to obtain a loan. In contrast, our focus is on generating one good counterfactual per patient in order to reduce the cognitive load on a physician.
Our focus is on counterfactual generation as a means for explanation and interpretability.
%One area of prior work is generating a diverse set of counterfactuals that capture the many ways in which a specific input could be changed to yield a different output (e.g. in our setting there could be many different vital measurements whose change would impact ventilation.) 
% I think we can argue that doing optimization every time is inefficient in time, but also inefficient in using the data, because each optimization is done independently and you don't get the benefit of learning about the energy landscape across samples
% we want a learned patient representation to make more effective comparisons
Echoing the discussion in \Cref{sec:intro}, we highlight four key characteristics of a time-series counterfactual generation method, and how/if these are handled in other methods of CFs: 
\begin{enumerate}
\itemsep0em 
    \item It works on time series data.
    \item The counterfactuals are \emph{relevant}, i.e. the produced counterfactuals are similar to the input.
    \item The counterfactuals are \emph{plausible}, i.e. the produced counterfactuals look like realistic patients.
    \item The counterfactual perturbations are \emph{sparse}, i.e. they materially differ from the input patient in only a few coordinates.
\end{enumerate}

%4. High counterfactual validity, 
%4. The model is \emph{feed-forward}, and
%5. The model learns a latent representation of the data. See \Cref{sec:intro} for more details into each of these. 
The closest related work on generating counterfactuals to explain a blackbox model include \citep{dhurandhar2018explanations,joshi2019towards,delaney2020instance,mothilal2020explaining,xu2022counterfactual}.  
We compare the prior work on each desirable characteristic we listed above. \\

\textbf{{Time series counterfactuals:}} Among the previously mentioned approaches,~\citep{delaney2020instance} is the only work explicitly generating time series counterfactuals. The time series counterfactual is generated by perturbing the original data point as described in the next paragraph (Relevance). \\

\textbf{{Relevance:}} \citep{delaney2020instance} produces relevant points by directly searching for the nearest unlike neighbor (NUN) and then transforms them in the direction of the original point as far as it can without crossing the decision boundary. However, it is possible that another near neighbor would have been transformed substantially nearer to the original point than is the NUN. \citep{joshi2019towards} learns a latent embedding of the data, and in this space aims to find a nearby point on the opposite side, with the intuition that the VAE should give nearby embeddings to nearby patients. 
\citep{dhurandhar2018explanations, mothilal2020explaining} and produce counterfactuals by performing a search in the original Euclidian space, directly minimizing the distance between the input and the generated counterfactual.  \citep{xu2022counterfactual} works on a binary input space (sets of diagnosis codes), and searches for nearby vertices of the Boolean hypercube which flip the classification labels. Thus, the generated CFs are forced to be largely similar the the point from which they are derived, and the few altered features are directly responsible for the label change. \\

\textbf{{Plausibility:}} After identifying the nearest unlike neighbor to a given time series,~\citep{delaney2020instance} changes the `high importance' regions of the input with segments from the NUN. While often sensible, this CF generation approach has a major pitfall when it comes to plausibility: in many cases one cannot directly substitute a time series segment from one patient with that of another patient. 
For tabular data, the approach in~\citep{dhurandhar2018explanations, mothilal2020explaining} of searching for the decision boundary in the data space can result in implausible counterfactuals: e.g., while an SpO$_2$ reading of 105 is close to a patient with SpO$_2$ 98, the former is not realistic. For example, a healthy patient with a constant heart rate of 60bpm should not have a CF where a random segment is replaced by a heart rate ascending from 140 to 180, only to immediately jump back down to 60 afterward. 
\citep{joshi2019towards} ensures plausibility by training a VAE to approximate the data distribution and learn an embedding (latent) space. The algorithm optimizes a loss function to search over the latent space for a counterfactual.
\citep{xu2022counterfactual} posits that their method of only changing subsets which are both sufficient and necessary inherently induces plausibility. \\

\textbf{{Sparsity:}} The work of~\citep{delaney2020instance} defines sparsity in terms of the length of the modified data segment rather than in terms of number of features they touch. Thus, they attempt to find short perturbations to the time series that flip the label. While this fits nicely within their framework, it is specific to signals whose label is largely defined by short-duration events (e.g. a single arrhythmia) and is not as well suited for sparsely capturing long-term trends in a small number of signals. 
In~\citep{mothilal2020explaining}, the authors propose augmenting their base model with an explicit post-hoc sparsification step. To sparsify the generated counterfactuals, they perform a greedy coordinate descent until no further coordinates can be independently minimized without crossing the decision boundary.
Because~\citep{xu2022counterfactual} works on a binary input domain, sparsity and relevance coincide in their work and so their search for a small set of diagnosis codes that collectively flips the classifier output inherently induces sparsity. The remaining works did not specifically target sparsity. \\

% \textbf{{Stability:}} In section \ref{sec:intro} we define a stable method to be one that produces similar counterfactuals for similar patients. In the healthcare domain, we might say that two patients are similar if some notion of their health metrics is similar. E.g., patients who have a similar pattern in heart rate, etc. Note that this does not mean similarity as measured by a distance metric such as $\ell_2$ norm. An increase in heart rate by 5 and SpO$_2$ by 5 are very different counterfactuals. Since \citep{delaney2020instance},\citep{mothilal2020explaining},\citep{dhurandhar2018explanations} operate in the input space and minimize the distance to the counterfactual, they do not capture the notion of stability that we describe. Note that in all of these methods, inputs that are similar (in terms of the $\ell_2$ norm) produce similar counterfactuals -- however for a health application, similarity should capture more than just the $\ell_2$ norm.   

%\textbf{{Feed-forward approach:}} The prior works listed \citep{delaney2020instance},\citep{mothilal2020explaining}, \citep{dhurandhar2018explanations},\citep{joshi2019towards} all involve generating counterfactuals by optimization to search the input space (\citep{delaney2020instance},\citep{mothilal2020explaining}, \citep{dhurandhar2018explanations}) or a learned latent space \citep{joshi2019towards} - none of these in prior work are feed-forward approaches. 

%\textbf{{Using a learned representation:}} As described in the paragraph about stability, we want to capture a notion of patient similarity to produce high quality counterfactuals. Computing the distance in the input space is not sufficient to capture similarity. A learned patient representation can help make effective comparisons. Among the prior works, \citep{delaney2020instance},\citep{mothilal2020explaining} operate in the input space. \citep{dhurandhar2018explanations} uses representations learned by an autoencoder. \citep{joshi2019towards} is similar to our work in using a VAE to generate counterfactuals. 

% Compared to the prior work, our proposed method has all of the above desirable characteristic. Our method is based on a transformer-VAE model to generate time series counterfactuals. Our solution is a feed-forward approach that produces a counterfactual by sampling from the learned latent space to capture patient similarity. The latent space is learned to jointly optimize plausibility and counterfactual validity.   

% In \citep{delaney2020instance} the authors propose a method to generate time series counterfactuals by identifying the closest data point in the training set of the opposite class and perturbing high importance regions of the time series and substituting it with values from the identified data point. This however has a major pitfall in a health application - a part of the time series data from one patient can not be substituted with data from another patient. For e.g., if a patient has a rising heart rate (140-180) between time 10 and 12 hours, this cannot be appended to a patient whose heart rate was roughly flat (at 60). This method can produce counterfactuals that are not plausible. Further, this method is not stable since the region of high importance depends on each data point at test time 
% the approach is 


% \citep{mothilal2020explaining} and \citep{dhurandhar2018explanations} generate a counterfactual by minimizing the Eucledian distance between the input and the generated counterfactual. This can result in unrealistic counterfactuals, e.g., while an SpO$_2$ reading of 105 is close to a patient with SpO$_2$ 98, it is an unrealistic counterfactual. In \citep{joshi2019towards} the authors use a VAE to approximate the distribution of data. Given an input data point, gradient descent is performed on a counterfactual objective in the latent space until a counterfactual is reached. All these methods are alike in using an optimization based approach to generate a counterfactual whereas we use a feed-forward approach since the latent space of the CF VAE has learned the classifier boundary using stochastic gradient descent. Another distinction is that \citep{joshi2019towards}, \citep{mothilal2020explaining},\citep{dhurandhar2018explanations} do not generate time series counterfactuals, which is actually our interest.

% Prior work on generating time-series counterfactuals includes \citep{delaney2020instance} and \citep{tonekaboni2019explaining}. In \citep{delaney2020instance} for a given input time series, its nearest unlike neighbor (NUN) is identified. The input time series is then modified to contain the values of the NUN in regions of `high importance' identified by a feature attribution method. This approach while simple and intuitive, has a major pitfall that a part of the time series data from one patient can not be substituted with data from another patient. For e.g., if a patient has a rising heart rate (140-180) between time 10 and 12 hours, this cannot be appended to a patient whose heart rate was roughly flat (at 60). This method can result in counterfactuals that are not realistic. The work in \citep{tonekaboni2019explaining} involves generating synthetic time series and computing an importance matrix of the different time points and features based on the effect of changing the original input. This work however does not generate counterfactuals where the aim is to flip the decision of a classifier.   

We note that there are many alternative explainable approaches that do not utilize counterfactuals. For example, attribution-based approaches have been extensively explored in prior work.  Such methods seek to quantify the effect that each dimension has on the prediction, e.g., via integrated gradients~\citep{sundararajan2017axiomatic}. In a canonical approach, ~\citep{caruana2015intelligible} investigates Gaussian Additive Models to explain the extent to which each input feature predicts pneumonia risk. Other methods include LIME \citep{ribeiro2016should} and SHAP \citep{lundberg2017unified}. While these approaches are effective in identifying why a particular model makes a decision, their outputs may not be easy for non-experts to consume. Moreover, the ability to explain decisions in terms of specific alternative patient cases is an extremely good fit to the reasoning processes that underlie clinical decision-making, and is therefore attractive in clinical settings.

\iffalse
\subsection{Predicting in-hospital clinical events}

There is substantial prior work on predictive analytics using clinical datasets such as MIMIC III. Some representative examples include predicting pneumonia risk~\citep{caruana2015intelligible}, 
sepsis~\citep{henry2015targeted,raghu2017continuous,eswaran2019intervention}
c diff~\citep{wiens2012patient}
and the more general
prediction of disease onset~\citep{razavian2016multi}.
We introduce a new home hospital problem: rank patients based on their time to critical intervention. 
 We partition the set of interventions into two types: those that can only be administered in the hospital and the rest.  Our goal is to use historical data about past interventions to rank new patients according to the expected time to an in-hospital intervention.  
We propose a solution based on using transformers.
This is an impactful problem that the community should continue to investigate.

\jrnote{This section is not good. We are doing intervention prediction. Which prior work is our method most closely-related to? How does our solution approach differ from that prior work, if at all? What is the justification for our approach?}
\fi

% \jrnote{we also need to describe our temporal representation of slope-intercept, does it have any novel aspects? Have others used this before? Not clear which section this goes in}

\iffalse
\subsection{Patient ranking}
The closest work to this is \citep{caruana1996using} where the authors seek to to rank pneumonia patients according to their mortality risk. The lowest ranked patients are evaluated as candidates for home treatment. The model is further trained on a secondary task to predict lab outcomes to learn better representations for the ranking task. However, subsequent work~\citep{caruana2015intelligible} identified concerns with using this intervention-oblivious model to assess risk. Similarly,~\citep{jing2020machine} attempts to prioritize patients according to the probability that a quick intervention can prevent their death. In contrast, our task is to rank patients based on time to in-hospital intervention. The problem is conceptually different from mortality prediction, or ranking based on the (reduction of the) risk of mortality. The general task we propose is to rank patients based on the time to \textit{any} in-hospital-only intervention which can be used to identify home-hospital candidates.  

\citep{barnes2016real},\citep{bishop2021improving} rank patients based on their likelihood of being discharged from the hospital. Related to this, a possible interpretation of the patient ranking problem is \textit{predicting} hospital length of stay since, in principle, patients that will be discharged sooner can be ranked higher than those with longer stays.~\citep{purushotham2017benchmark,gentimis2017predicting} predict critical-care unit length of stay in MIMIC-III and~\citep{lajevardi2021novel} predict length of stay in both critical and home hospital care.  Our work differs in that we are not trying to rank based on the time predict length of stay. Home hospital programs have evolved to the point where more previously in-hospital-only interventions can now be performed at home. The time to in-hospital-only interventions are what drive the ranking in this paper.
\fi
% \jrnote{Since this is a key task we are solving I think we need to discuss if it is novel or not and how existing approaches compare to ours.}

\iffalse
\subsection{Predicting Time to Intervention}
Predicting time to intervention in the ICU is a critical problem and helps allocate resources effectively and has been studied in prior work. The task in prior work is predicting whether an intervention will be needed in the next x hours. \citep{ghassemi2017predicting} train autoregressive state space models to predict if interventions such as vasopressor,ventilator are needed in the next 8 hours. \citep{suresh2017clinical} improves on the results in the previous work and makes predictions about interventions needed in the next 6 hours. \citep{wang2020mimic} consists of several benchmark tasks on MIMIC III including a 4 class classification task (wean on, wean off, stay on, stay off) for interventions in ICU patients. The paper explores different classical ML and deep feature learning models such as CNN and LSTM. More recently, \citep{lorenzen2021using} used a Random Forest model to predict ICU ventilator use during the COVID-19 pandemic.  
While the focus of this paper is not to develop a model predicting time to intervention, it is related to the ranking task that we frame. Time to the next critical-intervention is used to determine the ground truth ranking of patients. Another distinction is that prior work is that for the home-hospital problem, we would be ranking patients based on the time to \textit{any} hospital-only intervention. 
\fi
